# Supplementary material for: A simple and general approach for reversible condensation polymerization with cyclization
Source: arXiv:2302.04483 source file (2023-02-09)
Supplement: Supplementary file 1 [file SI.pdf]

# A simple and general approach for reversible condensation polymerization with cyclization: Supporting Information

Michael Lang<sup>\*,†</sup> and Kiran Suresh Kumar<sup>†,‡</sup>

*<sup>†</sup>Institut Theorie der Polymere, Leibniz Institut für Polymerforschung Dresden, Hohe Straße 6, 01069 Dresden, Germany*

*<sup>‡</sup>Institut für Theoretische Physik, Technische Universität Dresden, Zellescher Weg 17, 01069 Dresden, Germany*

E-mail: lang@ipfdd.de

## Monte Carlo simulations

We perform Monte-Carlo simulations to connect reversibly a large set of  $M \geq 10^6$  molecules, each containing  $f$  sticky groups. For simplification, we address only the case of an exclusive pairwise binding of the sticky groups. Let  $c_e$  denote the number concentration of “external” reactive groups per unit volume leading to inter-molecular bonds, while  $c_i$  is the “intra-molecular” number concentration per unit volume of a single open sticker of the same macromonomer in the vicinity of the selected sticky group, see equation (10) of the main text. Our aim is to discuss the general features of the competition between intra-molecular and inter-molecular reactions in a linear polymerization. We further use  $j$  to denote the number of closed stickers of the macromonomer,  $\tau$  for the dimensionless renormalized “lifetime” of the bond and  $V$  for the “reaction volume”, i.e. the volume around a given sticker in which a nearby sticker binds to it.

The simulations are based upon the following algorithm:

1. Pick randomly one sticky group.
2. If this group is connected, try to break the bond with probability  $1/\tau$ . Otherwise (group is not connected), try to create a bond with probability  $(c_e + (f - j - 1) c_i) V$ .
3. Repeat  $Mf$  times the above steps 1-2 to complete one Monte Carlo step (MCS).
4. Determine weight fractions  $w_j$  of molecules with  $j$  stickers closed, analyze distribution of cyclic species among the molecules, and compute  $p$  at the end of each MCS.

The coefficient  $f - j - 1$  for intra-molecular reactions counts the number of open stickers minus one, which is the number of possible intra-molecular reactions per picked open sticker of a macromonomer. This is sufficient for the case of exclusive loop formation, for loop formation only within a given macromonomer, or when analyzing linear polymerization where each chain has just one end. If networks are formed, the connected reactive groups inside the current aggregate further away must be considered too. How this can be implemented in approximate manner will be discussed in subsequent work. Note that step two of the algorithm limits our computations to parameters that satisfy  $(c_e + (f - j - 1) c_i) V < 1$ .

Above, we have used quotation marks for the lifetime, since we consider an effective binding energy  $\epsilon$  that is the difference between the detachment barrier energy and the effective attachment barrier energy. It is this energy difference that accounts for the frequency of closed and open stickers in an equilibrium situation, while the true time dependence of dynamic processes is related to the attachment and detachment energy barriers<sup>1</sup>. This is accounted for by selecting the attachment time as unit time of our algorithm. Thus, our algorithm refers to a reaction constant

$$K = \tau V \tag{1}$$

where  $\tau$  refers to the dimensionless renormalized “lifetime” of the bond with respect to the attachment time. Note that this reaction constant is defined as the concentration ratio

of reaction products and reactants with their corresponding powers, see also equation (2) of the main text. As further simplification, we choose the unit volume,  $V = 1$ , as the reaction volume, since a different choice only renormalizes the reaction constant.

Our simulations start with all stickers open and we equilibrate the system for at least  $20\tau$  MCS. Note that  $\tau$  can be considered as the “relaxation time” of the system, since bonds are exchanged on this particular timescale and conversion relaxes exponentially towards its asymptotic value. After this equilibration step, data is sampled for at least  $100\tau$  and typically, ten conformations per time interval  $\tau$  are analyzed and averaged. Since  $M \geq 10^6$ , the statistical error of the simulation data is usually below  $10^{-4}$ .

## Numerical solutions

In the main part of this work, detailed balance conditions of the form

$$a_j w_j = b_k w_k \quad (2)$$

for all possible transitions between molecules with  $j$  or  $k$  bonds are derived. Here,  $a_j$  and  $b_k$  can be coefficients or functions of the reaction constant  $K$  and conversion  $p$ . Typically, there are  $f$  of these equations relating  $j = k + 1$  (and  $j = k + 2$  in case of loop formation) with  $k$ . These detailed balance conditions will be given explicitly for each particular model system.

To solve the set of balance equations, we require two more relations, which are the normalization condition of the weight fractions

$$\sum_{j=0}^f w_j = 1, \quad (3)$$

and conversion

$$p = \sum_{j=1}^f j w_j / f. \quad (4)$$

Altogether, we obtain  $f + 2$  equations for  $f + 2$  unknowns (the  $f + 1$  weight fractions

$w_j$  and  $p$ ), plus an infinite set of balance equations for the loop size distribution that can be boiled down to a single relation between  $w_0$  and the weight fraction of loops,  $\omega$ , see section *Homopolymerization with cyclization (case 1)*. In principle, this allows to obtain an analytical solution for the set of balance equations, however, these are practicable only in some special cases (e.g. smallest loop model).

Therefore, we use the following numerical recursion to obtain numerically exact solutions:

**Step 0:** Set  $w_j = (f + 1)^{-1}$  and  $p = 1/2$  as “arbitrary” initial conditions.

**Step 1:** Compute improved estimates for  $w_j$  and loops based upon the distribution of  $w_j$  of the preceding recursion step using detailed balance conditions; renormalize  $w_j$  such that these satisfy equation (3) and compute an improved estimate of  $p$  through equation (4).

**Step 2:** Repeat Step 1 until a desired accuracy limit has been reached. In our case, the difference of  $p$  between two subsequent recursion steps had to drop below a very small threshold (typically  $10^{-6}/K^2$ ) to accept the current set of  $w_j$  as an approximation for the analytical solution.

The above scheme was successfully tested against the analytical solutions of loop free model systems and of models with exclusive loop formation, see section *General aspects of inter-and intra-molecular reactions*. These analytical solutions were also used to test the simulation. All numerical solutions for the mixed cases (inter- and intramolecular bonds) we have studied agree within numerical accuracy with the corresponding simulation data.

The supporting information (SI) contains a minimum example for the recursive computations necessary to solve case 1. To keep the example simple, additional checks for consistency, numerical stability, etc., were omitted as these are beyond the scope of the manuscript. Therefore, numerical data as obtained from a similar algorithm should be considered with care. Sign changes, oscillatory solutions, or abrupt jumps of  $p_{\text{lin}}$  or  $\omega$  are definite signatures of numerical instabilities and corresponding computations have to be dropped. In the example of the SI,  $c_e$  is adjusted while  $K$  and  $c_i$  are kept fixed, however,

any of these variables (or several of these) could be modified within the computation loop.

## References

- (1) Rubinstein, M.; Semenov, A. N. Thermoreversible Gelation in Solutions of Associative Polymers. 2. Dynamics. *Macromolecules* **1998**, *31*, 1386–1397.

## Figures

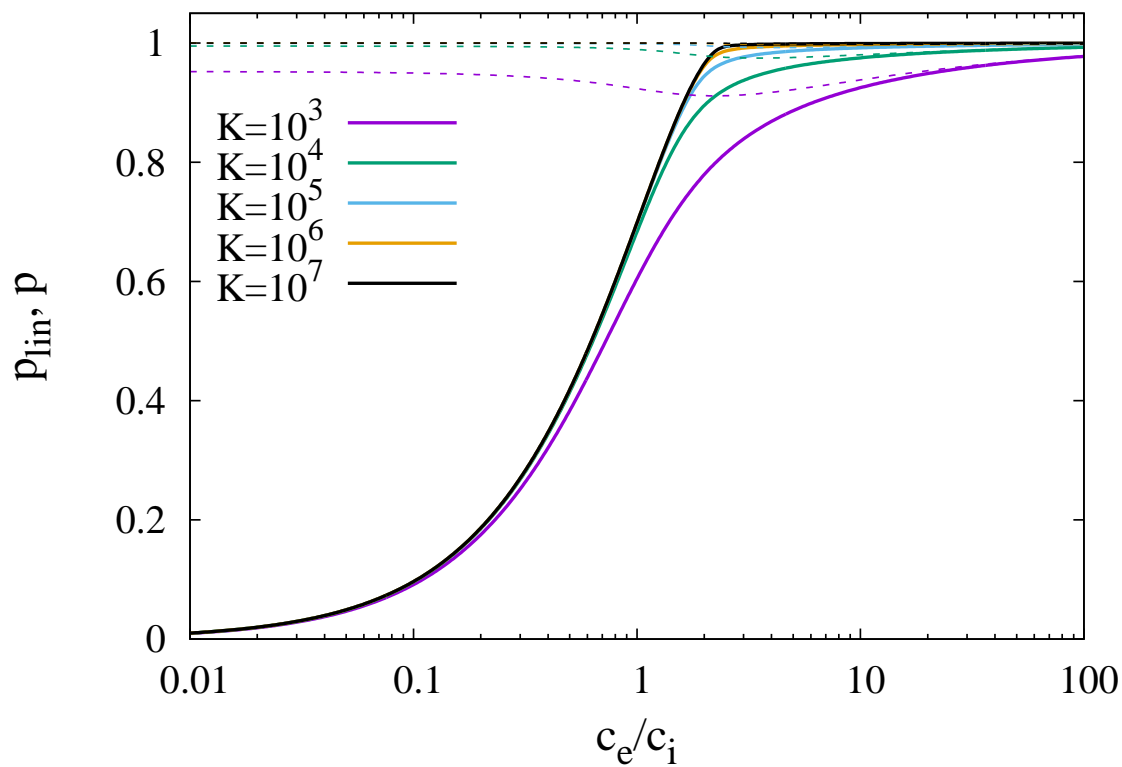

Figure S1:  $p_{lin}$  (solid lines) as a function of  $c_e/c_i$  for a range of reaction constants with  $c_i = 10^{-2}$  compared with  $p$  (dashed lines).

```

Program example
implicit none

integer i,j,g                ! run variables of do loops
Parameter (g=1000)          ! largest loop that is considered
double precision omega       ! weight fraction of loops
double precision ce          ! external concentration
double precision ci          ! internal concentration
double precision p           ! conversion
double precision p_lin       ! conversion of linear chains
double precision w(0:2)      ! weight fractions of monomers with j closed stickers
double precision p_old       ! conversion of previous step - is used as criterion to stop the current recursion
double precision sum_L,sum_w ! sums over number fraction distribution / weight fractions of monomers
double precision low         ! termination criterion for recursion
double precision nk          ! variable used for summation over loops
double precision K           ! reaction constant

K = 1000.0                  ! set reaction constant
low = 0.000001/K**2        ! termination condition for conversion - needs to be adjusted for large K
write(*,*) low

open(10,file = 'K1000.dat')

do i = 0,500
  write(*,*) i              ! show progress on screen
  ci = 0.01                 ! initialization of concentrations
  ce = ci*1.02**i/100.0

  p = 0.5                   ! arbitrary initialization of w_j and p
  w(0) = 0.33
  w(1) = 0.33
  w(2) = 0.33
  p_lin = p

1  p_old = p                 ! repeat from here, if not yet converging
  nk = 1.0
  sum_L = nk
  do j = 2, g
    nk = nk*p_lin
    sum_L = sum_L + nk*DBLE(j)**(-1.5) ! this provides sum term in equation (28)
  enddo

  omega = 2.0*ci*w(0)*K*sum_L        ! equation (28) with equation (12) for weight fraction of smallest loops
  w(1) = 4.0*ce*(1.0-p)*w(0)*K      ! equation (13)
  w(2) = ce*(1.0-p)*w(1)*K + omega   ! equation (14)

  sum_w = w(0) + w(1) + w(2)         ! now enforce normalization
  w(0) = w(0)/sum_w
  w(1) = w(1)/sum_w
  w(2) = w(2)/sum_w
  omega = omega/sum_w

  p = w(2) + 0.5*w(1)               ! compute conversion, equation (82)
  p_lin = (p-omega)/(1.0-omega)      ! equation (16)

  if (abs(p-p_old) .gt. low) goto 1  ! check whether numerical solution converges

  write(10,*) i,ci,ce,p,K,p_lin,omega
enddo

2  close(10)
end

```

Figure S2: Fortran example code for computing a numerical solution
